# Supplementary material for: Nonlocal Correlation Mediated by Weyl Orbits
Source: arXiv:2002.00148 source file (2020-02-01)
Supplement: Supplementary file 1 [file Supplementary_Materials.pdf]

# Supplementary Materials for

## Nonlocal Correlation Mediated by Weyl Orbits

Zhe Hou[1] and Qing-Feng Sun[1,2,3]*

1 International Center for Quantum Materials, School of Physics, Peking University, Beijing 100871, China.

2 Collaborative Innovation Center of Quantum Matter, Beijing 100871, China.

3 CAS Center for Excellence in Topological Quantum Computation, University of Chinese Academy of Sciences, Beijing 100190, China.

Correspondence to: sunqf@pku.edu.cn

## 1. Method for calculating the density of states

In this section we provide the numerical method for calculating the density of states (DOS) inside the Weyl semimetal (WSM) slab. We first rewrite the Weyl Hamiltonian $\widehat{H}$ in the tight-binding form:

$$\widehat{H} = \sum_i [c_i^\dagger T_0 c_i + c_i^\dagger T_x c_{i+\delta\mathbf{x}} + c_i^\dagger T_y c_{i+\delta\mathbf{y}} + c_i^\dagger T_z c_{i+\delta\mathbf{z}} + \text{H.c.}] \qquad \text{(S1)}$$

by performing the Fourier transformation: $c_i = \frac{1}{\sqrt{N}} \sum_{\mathbf{k}} e^{i\mathbf{k}\cdot\mathbf{r}_i} c_{\mathbf{k}}$ with $c_i = (c_{i\uparrow}, c_{i\downarrow})^T$. Here $c_{i\uparrow}(c_{i\downarrow})$ is the annihilation operator at site $i$ with spin ↑ (↓), $N$ is the total site number of the system and $\mathbf{r}_i$ is the position of site $i$. The $T$-matrice in Eq. (S1) are :

$$T_0 = \begin{pmatrix} 2t_z + 2\gamma & 0 \\ 0 & -2t_z - 2\gamma \end{pmatrix}, \quad T_x = \begin{pmatrix} -t_z/2 & t_x/2i \\ t_x/2i & t_z/2 \end{pmatrix}, \quad T_y = \begin{pmatrix} -t_z/2 & -t_y/2 \\ t_y/2 & t_z/2 \end{pmatrix},$$

$$\text{and } T_z = \begin{pmatrix} -t_z/2 & 0 \\ 0 & t_z/2 \end{pmatrix}. \qquad \text{(S2)}$$

In calculating the DOS, we divide the slab into three regions: left infinitely-long nanoribbon (with Hamiltonian $H_L$), the central region (with Hamiltonian $H_C$), and right infinitely-long nanoribbon (with Hamiltonian $H_R$). The two infinitely-long nanoribbons satisfy the Hamiltonian Eq. (S1) and have a surface Green's function $\mathbf{g}_{L(R)}^s(E)$ for the left (right) terminal. The central region contains the surface potential wells (PWs) $U(\mathbf{r})$ and its Green's function can be obtained as: $\mathbf{G}_C^r(E) = \left[(E + \eta t)\mathbf{I} - H_C - \sum_{m=L,R} \Sigma_m^r\right]^{-1}$. Here $\eta$ is an infinitely-small imaginary number, and $\Sigma_m^r$ is the self-energy of terminal $m$ which is calculated as: $\Sigma_m^r = H_{Cm}\mathbf{g}_m^s H_{mC}$ where $H_{Cm}(H_{mC})$ denotes the coupling between the central region and terminal $m$. The DOS at site $i$ in the central region is obtained by taking the imaginary part of the Green's function:

$$\rho_i(E) = -\text{Im}\mathbf{G}_C^r(i, E)/\pi. \qquad \text{(S3)}$$

In the calculations, we set the imaginary number to $\eta = 0.001\text{i}$.

## 2. Method for calculating the transmission coefficients

In this section we provide the detailed numerical method to calculate the transmission coefficients in the six-terminal system combined with an infinitely-long WSM nanoribbon and four normal metal electrodes, as shown with Fig. 3(a) in the main text. The normal metal can be described by a tight-binding Hamiltonian $H_{NM} = \sum_{i,\sigma} E_0 a_{i\sigma}^\dagger a_{i\sigma} + t_{\text{NM}} \sum_{<ij>,\sigma} a_{i\sigma}^\dagger a_{j\sigma}$, with $a_{i\sigma}^\dagger(a_{i\sigma})$ the creation (annihilation) operator at site $i$ with spin $\sigma$, $E_0$ the on-site energy, and $t_{\text{NM}}$ the nearest hopping amplitude. The coupling between the normal metal and the WSM nanoribbon can be described with $H_{\text{coupl}} = t_{\text{coupl}} \sum_{i\in NM, j\in WSM,\sigma} a_{i\sigma}^\dagger c_{j,\sigma} + \text{H.c.}$ with $t_{\text{coupl}}$ the coupling strength. Similar to section (1), we divide the transport system into six terminals labelled by the index $m$= front, bottom, 1, 2, 3, 4, and a central region with Hamiltonian $H_C$. By calculating the self-energies $\Sigma_m^r$ of the six terminals, the retarded Green's function of the central region is obtained as $\widetilde{\boldsymbol{G}}_C^r(E) = [(E + \eta t)\mathbf{I} - H_C - \sum_m \Sigma_m^r]^{-1}$. The transmission coefficients $T_{mn}$ from terminal $n$ to terminal $m$ can be obtained by *(1)*:

$$T_{mn}(E) = \text{Tr}[\Gamma_m(E)\widetilde{\boldsymbol{G}}_C^r(E)\Gamma_n(E)\widetilde{\boldsymbol{G}}_C^a(E)], \qquad \text{(S4)}$$

where $\Gamma_m(E) = i[\Sigma_m^r - (\Sigma_m^r)^\dagger]$ is the line-width function for terminal $m$, and $\widetilde{\boldsymbol{G}}_C^a(E) = \left[\widetilde{\boldsymbol{G}}_C^r(E)\right]^\dagger$ is the advanced Green's function of the central region. In the real calculations, we set $E_0 = 0, t_{\text{NM}} = t$, and $t_{\text{coupl}} = t$.

After knowing all the transmission coefficients $T_{mn}$ in the six-terminal system, the current flowing into terminal $m$ is calculated by using the Landauer-Büttiker formula *(2)*:

$$I_m = \frac{e^2}{h}\sum_{n\neq m} T_{mn}[V_m - V_n] \quad \text{(S5)}$$

where $V_m$ is the voltage applied in terminal $m$.

### 3. The wave-function evolution on the Weyl orbit

In the main text we describe the real-space trajectory of the Weyl fermions in the WSM slab under the drive of the PWs. In this section we plot the wave-function evolution of the Weyl orbit to see how the wave-function is pumped from the top surface into the bottom one. In Fig. S1A we select six points on the Weyl orbit and plot their corresponding wave-functions in Fig. S1B. For the top surface state 1, its wave-function is localized on the top layer and decays quickly into zero after one-layer distance away from the surface. Under the drive of the top PW, the wave-function gradually evolve into state 2 with its broadening about two or three layers long. Further driving the wave-function, the surface state is pushed out of the topological region connected by the two Weyl nodes $\mathbf{K}_{\pm}$ and becomes the bulk state 3. Here the wave-function is distributed over the whole body of the WSM slab with few amplitudes permeating into the bottom surface. Once the bottom PW is placed, the local electrostatic force will continue driving the wave-function 3 by acting on its bottom surface part and then the wave-function is pumped into states 4, 5 and 6 sequentially. Finally, the top surface state 1 is pumped into the bottom surface state 6 under the assistance of both the top/bottom PWs.

In the calculations, we set the distance between the two Weyl nodes to the maximum value $\pi/a$ by fixing $\gamma = 0$, so that the broadenings of the surface states yield the minimum values *(3)* (less than three layers, see Fig. S1B). What's more, the slab thickness is set to $N_y = 20$ which makes the coupling between the top and bottom surface states infinitely-small, so the coupling regime of the surface states can be excluded in explaining the nonlocal correlation presented in the main text.

### 4. The DOS response in the central section of the WSM slab

In Fig.2(e-g) of the main text, we show the DOS versus the site indexes $i$, where the site $i = i_z + (i_y - 1)N_z$ counts from the left to the right and then from the bottom to the top. Fig.S2 shows the same DOS change $|\rho_{\mathrm{b}} - \rho_{\mathrm{no}}|$ and $|\rho_{\mathrm{tb}} - \rho_{\mathrm{t}}|$ versus the site $(i_z, i_y)$. But here the DOS is represented by color.

### 5. A designed experimental device for detecting the nonlocal transport signal

To give an experimentally detectable signal for the nonlocal transport discussed in the main text, we design a transport device in Fig. S3A. Similar to a Coulomb drag system, we make the front and back terminals grounded, pour a constant current $I$ in terminal 1 and 4, and connect an external voltmeter between terminal 2 and 3 to measure the responsive voltage $V_{23} \equiv V_2 - V_3$. We then define the nonlocal resistance $\rho_{NL} \equiv \frac{V_{23}}{I}$ as an experimental observable. Fig. S3B shows the calculated nonlocal resistance as a function of the Fermi energy $E_f$ (relative to the energy of the Weyl nodes) by using the Landauer-Büttiker formula in Eq. (S5). The result shows that the nonlocal resistance is greatly enhanced once the top/bottom PWs are both placed on the slab surfaces. The dramatic resistance peak at $E = 0.186t$ implies the Weyl bridge state. These observations can serve as evidence for verifying the nonlocal correlation mediated by the Weyl orbit in experiments.

### 6. A semi-classical description

In this section we give a semi-classical description on the trajectories of the Weyl fermion confined by the top/bottom PWs in an infinitely large WSM slab. The Hamiltonian of the WSM (in the momentum space) is $H(\mathbf{k}) = t\sigma_z\big(2 + \gamma - \cos k_x a - \cos k_y a - \cos k_z a\big) + t\sigma_x \sin k_x a + t\sigma_y \sin k_y a$. We first consider a continuous model to describe the Weyl orbit. Between the two Weyl nodes, the surface states can be described by an effective Hamiltonian or dispersion *(3)*:

$$E = \pm\hbar v k_x, \quad -k_0 < k_z < k_0. \tag{S6}$$

Here $\pm v$ is the group velocity of the bottom (top) surface states, and $v = ta/\hbar$ under the tight-binding model parameters. The bulk states near the Weyl nodes can be described by the dispersion:

$$E = \hbar\sqrt{v^2 k_x^2 + v_z^2 (k_z \pm k_0)^2 + v^2 k_{y0}^2}, \qquad |k_z| > k_0. \tag{S7}$$

Here the Fermi velocity $v_z = ta(\sin k_0 a)/\hbar$ is obtained by expanding $H(\mathbf{k})$ around the Weyl nodes, and $k_{y0}$ is the minimum wave-vector in the $y$ direction which can be approximated as $\pi/\big(N_y + 1\big)a$.

We consider the Weyl fermion trapped inside the top PW. Its semi-classical equations of motion can be written as:

$$\begin{aligned} \mathbf{\Pi} &= \partial_{\boldsymbol{k}} E(\mathbf{k})/\hbar, \\ \hbar d\boldsymbol{k}/dt &= \mathbf{F} = -\partial_{\boldsymbol{r}} U(\mathbf{r}). \end{aligned} \tag{S8}$$

Where $\mathbf{\Pi}$ is the semi-classical velocity, and the effect of the Berry curvature which arises from the multiband property of the band structure has been ignored. More specifically, Eq. (S8) can be rewritten into the following two-component forms:

$$\begin{aligned} \Pi_x = \partial_{k_x} E(\mathbf{k})/\hbar,\ \Pi_z = \partial_{k_z} E(\mathbf{k})/\hbar; \\ \hbar dk_x/dt = -2a_x x,\ \hbar dk_z/dt = -2a_z z. \end{aligned} \tag{S9}$$

Combining the above equations and the initial position $\mathbf{r}_0 = (x_0, z_0)$ and the initial wave-vector $\mathbf{k}_0 = (k_{x0}, k_{z0})$ at time $t = 0$, the trajectory of the Weyl fermions inside the PW can be hence solved.

Next let us consider one specific trajectory which is closed in both real and momentum space, and forms the Weyl bridge state. We consider that the Weyl fermion is incident from the position (1) on the top surface (see the planform of the WSM slab in Fig. S4A), i.e. incident from the bulk state with initial position $(r_0, 0)$ and initial wave-vector $(0, k_{z0})$ (see the corresponding momentum position in Fig. S4B). Once the Weyl fermion is captured by the PW, its real-space trajectory will deflect due to the attractive electrostatic force, and then arrives at position (2). The Weyl fermion thus migrates to the surface state and moves in $-x$ direction straightly with the velocity $(-v, 0)$. Here due to the persistent attraction in the $-z$ direction, the Weyl fermion moves leftwards in the momentum space from position (2) to position (3). If the change of the wave-vector $k_z$ during the motion from (1) to (3) satisfies:

$$\Delta k_z = k_0, \tag{S10}$$

where $k_0$ is the half-distance between the two Weyl nodes, the Weyl fermion will accomplish the following motion: moving from position (3) to (4) to get back to the bulk state, revolving in the real-space to immigrate to position (5), tunneling from the top surface to the bottom one, and then moving from (5) to (1) passing positions (6), (7) and (8) by repeating the motion (1-2-3-4-5). Finally, the Weyl fermion tunnels from the bottom surface to the top one and gets back to its original position. The real-space and momentum-space trajectories are therefore enclosed. If the phase accumulated during the enclosed loop is an integer multiples of $2\pi$, a constructive

interference inside the WSM slab happens, which results in a Weyl bridge state we discussed in the main text.

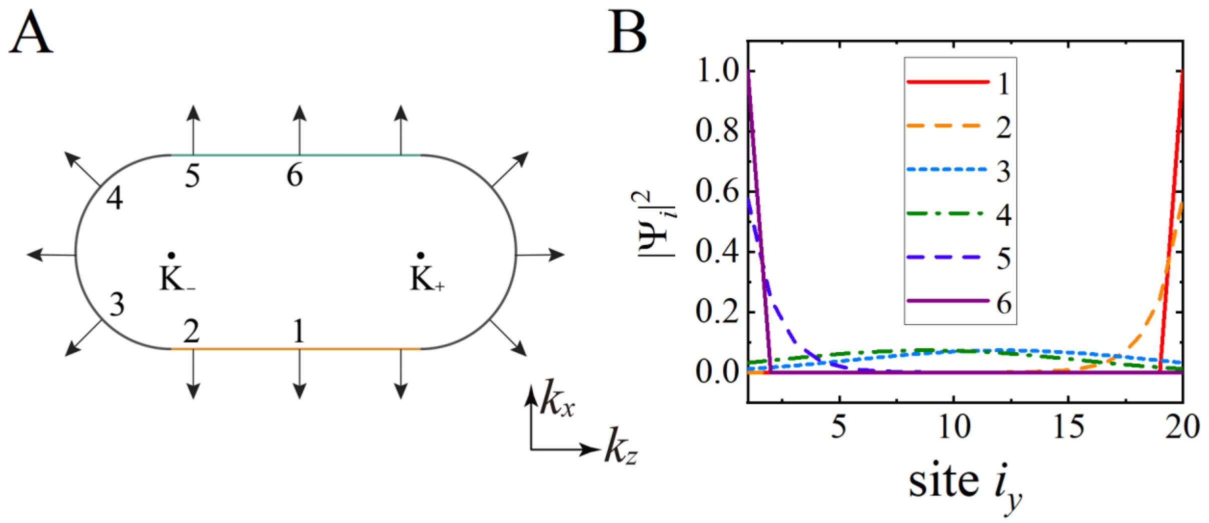


**Fig. S1. The wave-function evolutions in the Weyl orbit.** (**A**) The Weyl orbit with two Weyl nodes $\mathbf{K}_{\pm}$ enclosed inside. The yellow and green segments denote the top and bottom surface states, respectively, and the half-circles denote the bulk states. (**B**) The square modulus of the wave-function 1-6 picked from (A) distributing in the slab thickness direction $y$. The energy is chosen as $E = 0.2t$, and the wave-vectors $(k_x, k_z)$ of the state 1(6), 2(5), 3(4) are set as $\left(\pm\frac{0.201}{a}, 0\right)$, $\left(\pm\frac{0.201}{a}, -\frac{1.194}{a}\right)$, and $\left(\pm\frac{0.099}{a}, -\frac{1.696}{a}\right)$, respectively.

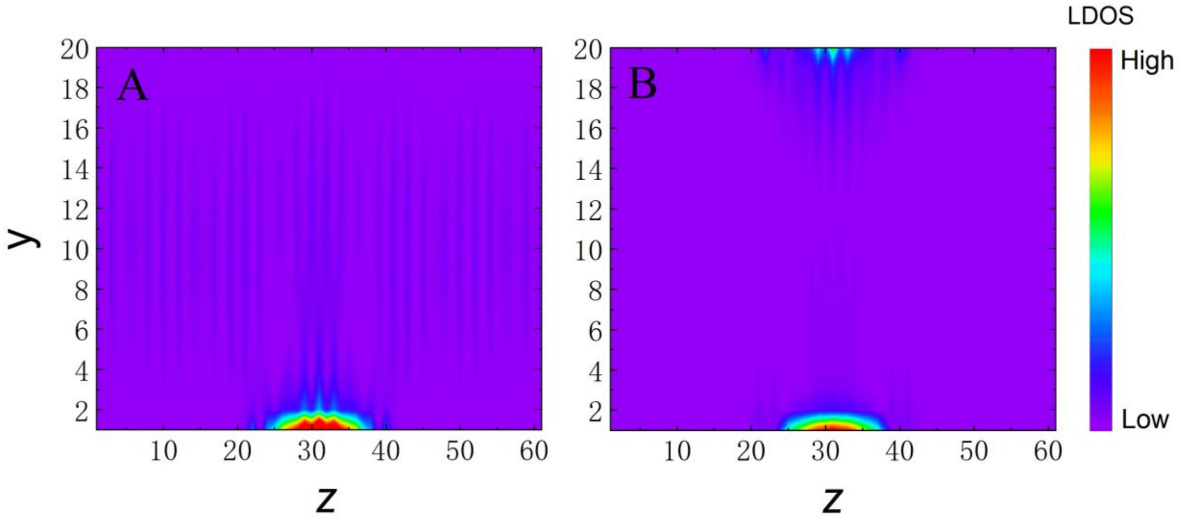


**Fig. S2. The DOS response in the central section of the WSM slab.** (**A**) and (**B**) The DOS change $|\rho_{\mathrm{b}} - \rho_{\mathrm{no}}|$ and $|\rho_{\mathrm{tb}} - \rho_{\mathrm{t}}|$. The parameters are the same as those in Fig. 2 of the main text.

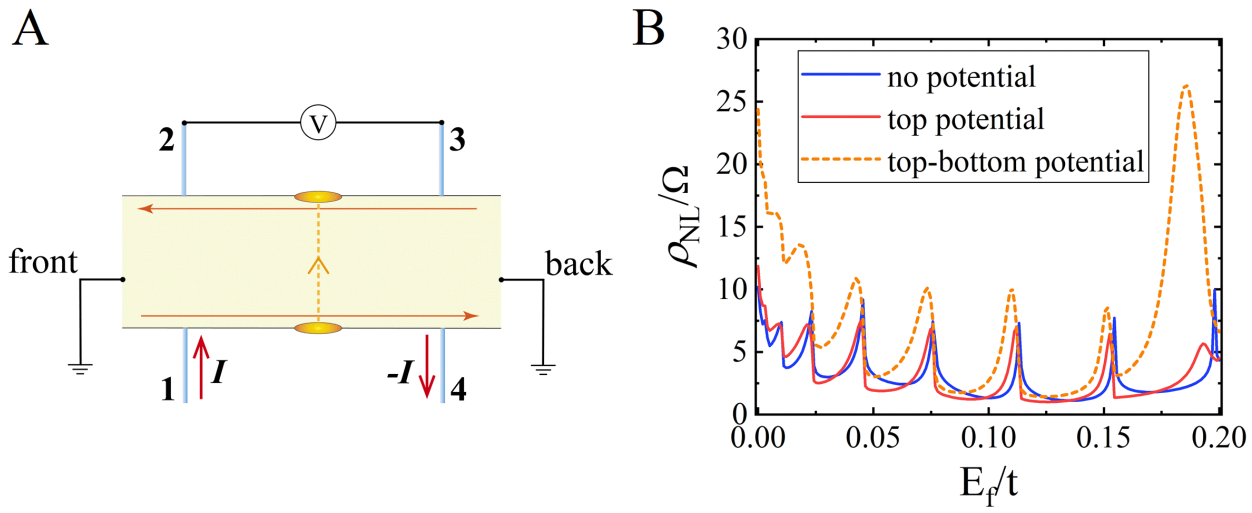


**Fig. S3. The experimental observable in the nonlocal transport in the WSM slab.** (**A**) A designed device for experimental observations. Here the front and back terminals are grounded, the terminal 1 and 4 are floured with a constant current $I$, and the terminal 2 and 3 are connected by an external voltmeter to detect the voltage response $V_{23} \equiv V_2 - V_3$. **(B)** The nonlocal resistance $\rho_{NL} \equiv V_{23}/I$ as a function of the Fermi surface $E_f$ (relative to the energy of Weyl nodes) in the six-terminal system.

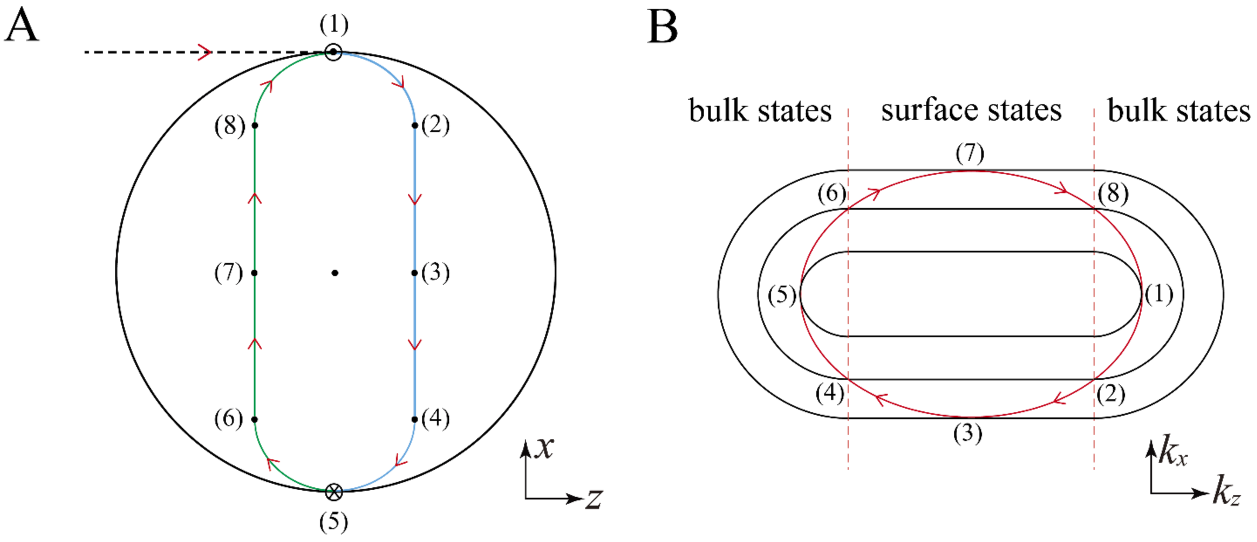


**Fig. S4. Semi-classical trajectories of the Weyl bridge state.** (**A**) Planform of the real-space trajectory for Weyl fermions confined in the WSM slab. The Weyl fermion first incomes from position (1) on the top surface, then passes the positions (2-8), and finally moves from position (8) back into the original position (1) to accomplish one enclosed loop which stretches across the whole WSM slab. Here the right blue curve denotes the trajectory on the top surface, and the left green curve denotes the trajectory on the bottom surface. On the connections of the top and bottom curves, the Weyl fermion realizes a tunneling between the top and bottom surfaces. (**B**) The enclosed trajectory (red curve) in the momentum-space, corresponding to positions (1-8) in (A). Here the black enclosed curves denote the iso-energetic Weyl orbits. Note that in Fig. 1(b) of the main text we only show one Weyl orbit with equal energy, but in the real motion the trajectory is not iso-energetic due to the confined potential and goes through many Weyl orbits, as shown in (B).

**Movie S1: A simulation on the natural phenomenon of lightning in a WSM slab.** Here the energy is scanned from $E = 0.14t$ to $E = 0.22t$. The PWs are placed on both the top and bottom surfaces. At $E = 0.186t$, a new resonant state confined by the top and bottom PWs appears, which forms a bridge linking the top and bottom surfaces and induces a body breakdown, similar to the lightning phenomenon. The parameters are the same as those in Fig. 2 in the main text.

## References

1. Z. Hou, Y. Xing, A.-M Guo, and Q.-F. Sun, Crossed Andreev effects in two-dimensional quantum Hall systems. Phys. Rev. B **94**, 064516 (2016).

2. S. Datta, “Double-barrier tunneling’’ in *Electronic Transport in Mesoscopic Systems* (Cambridge University Press, Cambridge, 1995), pp. 246-275.

3. C. M. Wang, H.-P. Sun, H.-Z. Lu, and X. C. Xie, 3D Quantum Hall Effect of Fermi Arcs in Topological Semimetals. Phys. Rev. Lett. **119**, 136806 (2017).
